# Supplementary material for: Orthogonal Time Frequency Space Modulation: A Discrete Zak Transform Approach
Source: arXiv:2106.12828 source file (2021-06-24)
Supplement: Supplementary file 1 [file appendix_frame.tex]

\begin{align}
		Z_{\mathbf{S}_x}[n,k] 	&= \frac{1} {\sqrt{K}}\sum_{l'=0}^{K-1} \sum_{m=0}^{K-1}\sum_{l=0}^{K-1} \langle x, y_{m,l} \rangle y[n+l'L-mL]e^{j2\pi\frac{l}{L}(n+l'L)}e^{-j2\pi\frac{k}{K}l'}\\
							&=  Z_y[n,k] \sum_{m=0}^{K-1}\sum_{l=0}^{K-1} \langle x, y_{m,l} \rangle e^{-j2\pi \left( \frac{k}{K}m -\frac{l}{L}n\right)}\\
							&= \sqrt{KL} Z_x[n,k] \left|Z_y[n,k]\right|^2
\end{align}
